# Supplementary material for: Bilinear CNNs for Fine-grained Visual Recognition
Source: arXiv:1504.07889 source file (2017-06-01)
Supplement: Supplementary file 1 [file patch_strip_suppl.tex]

\begin{figure}
\begin{center}
\setlength{\tabcolsep}{2pt}

\begin{tabular}{cc}
    D-Net & M-Net \\
    \includegraphics[width=0.485\linewidth]{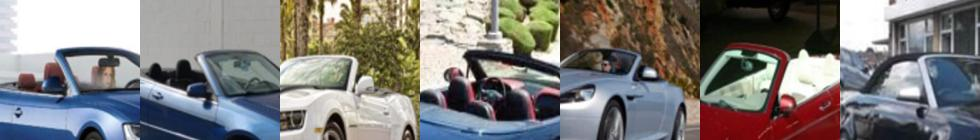} &         \includegraphics[width=0.485\linewidth]{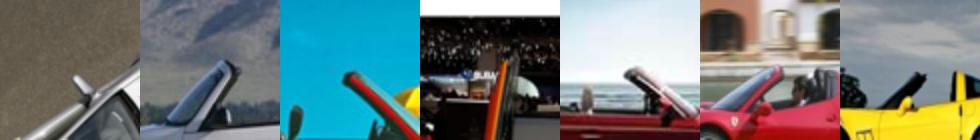} \\
    \includegraphics[width=0.485\linewidth]{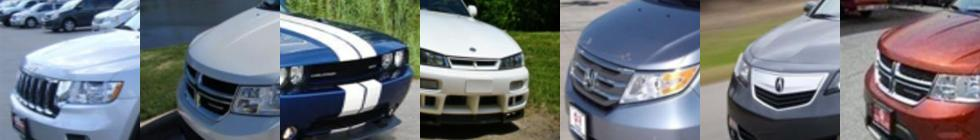} & \includegraphics[width=0.485\linewidth]{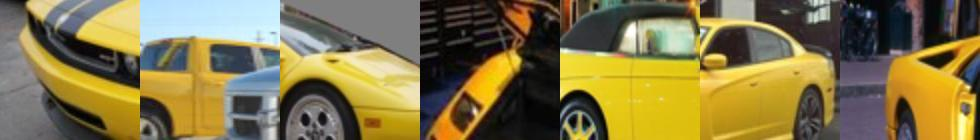} \\
    \includegraphics[width=0.485\linewidth]{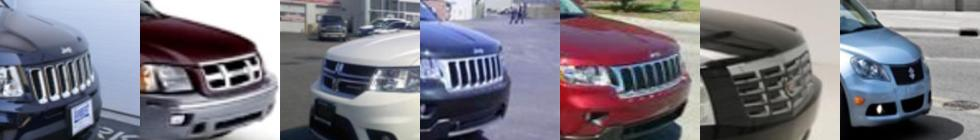} & \includegraphics[width=0.485\linewidth]{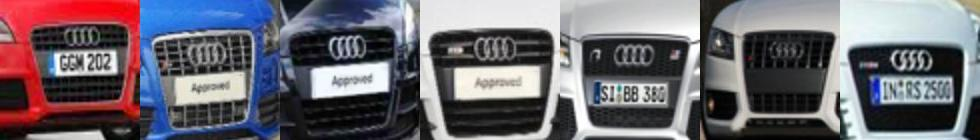} \\
    \includegraphics[width=0.485\linewidth]{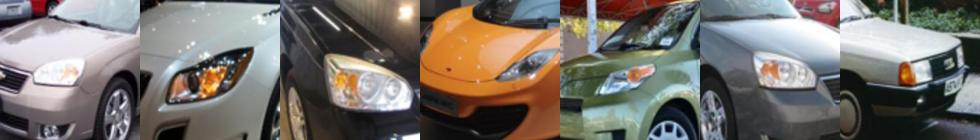} &  \includegraphics[width=0.485\linewidth]{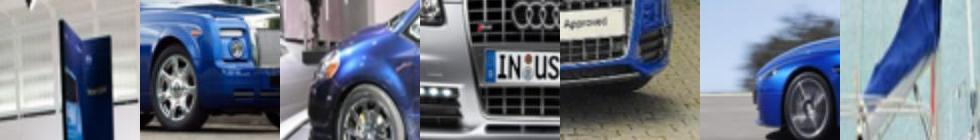}\\
    \includegraphics[width=0.485\linewidth]{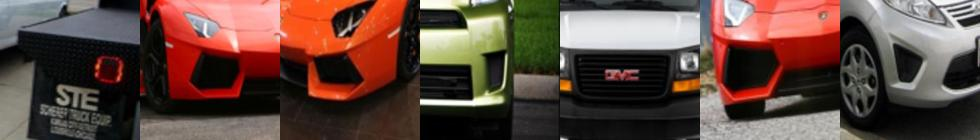} & \includegraphics[width=0.485\linewidth]{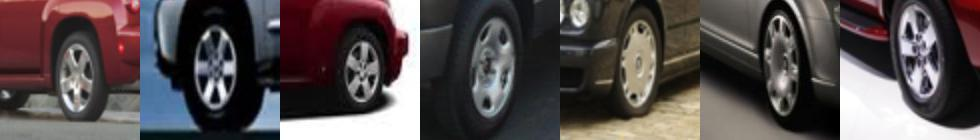}\\
    \includegraphics[width=0.485\linewidth]{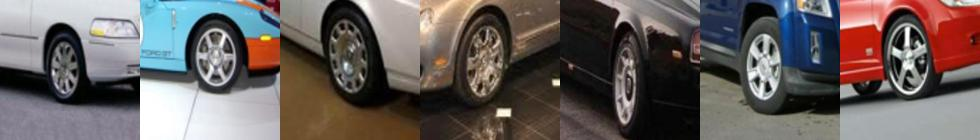} & \includegraphics[width=0.485\linewidth]{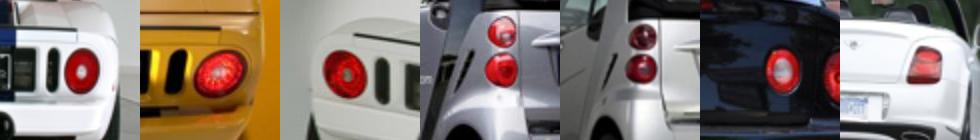}\\
    \includegraphics[width=0.485\linewidth]{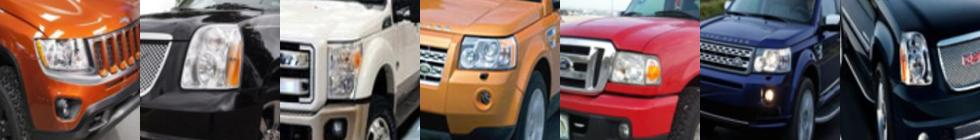} & \includegraphics[width=0.485\linewidth]{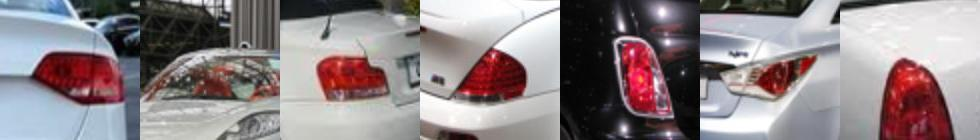}\\
    \includegraphics[width=0.485\linewidth]{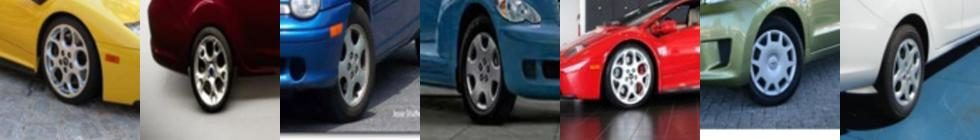} &  \includegraphics[width=0.485\linewidth]{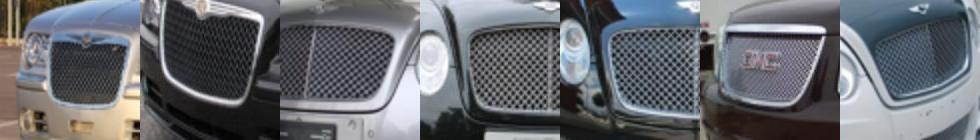}\\
    \includegraphics[width=0.485\linewidth]{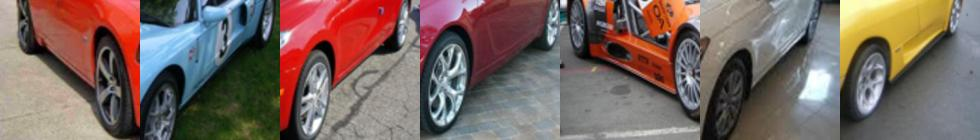} &  \includegraphics[width=0.485\linewidth]{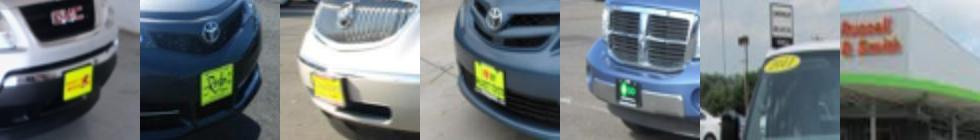}\\
    \end{tabular}
    \caption{\label{fig:bcnn-vis} Patches with the highest activations for several filters of the fine-tuned BCNN(D, M) model on the Cars dataset. We can clearly observe common patterns such as convertibles\textit{(top row, D-Net and M-Net)}, front bumpers and wheels \textit{(D-Net rows 2, 3, 8 and 9)}, various styles of tail lights \textit{(M-Net, rows 6 and 7)}, specific company logos as a pattern \textit{(M-Net row 3)}, a specific colour \textit{(M-Net rows 2 and 4)} etc. }
    \end{center}
    \end{figure}

\begin{figure}
\begin{center}
\setlength{\tabcolsep}{2pt}

\begin{tabular}{cc}
    D-Net & M-Net \\
    \includegraphics[width=0.485\linewidth]{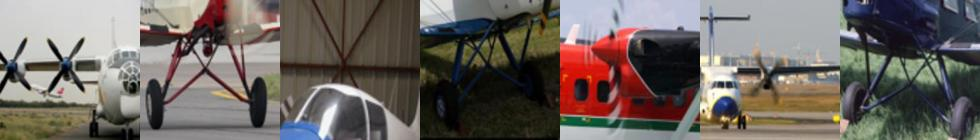} &         \includegraphics[width=0.485\linewidth]{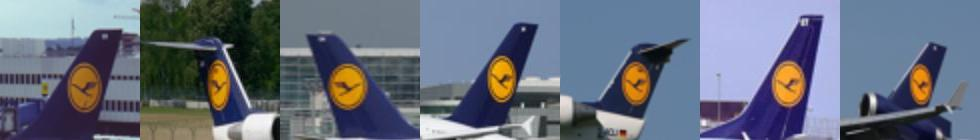} \\
    \includegraphics[width=0.485\linewidth]{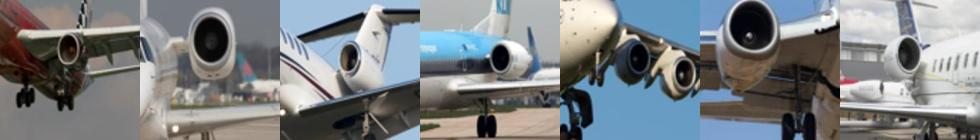} & \includegraphics[width=0.485\linewidth]{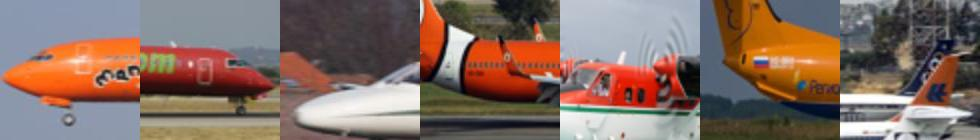} \\
    \includegraphics[width=0.485\linewidth]{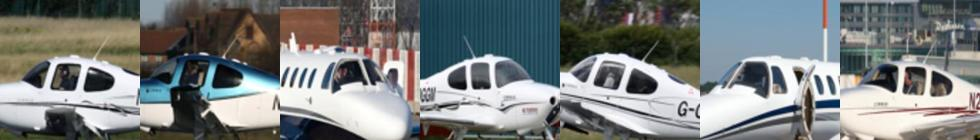} & \includegraphics[width=0.485\linewidth]{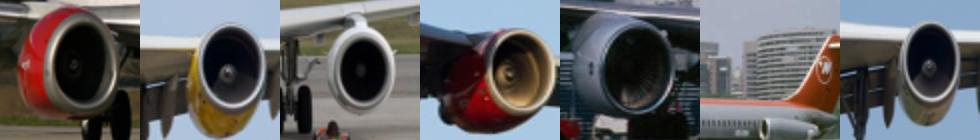} \\
    \includegraphics[width=0.485\linewidth]{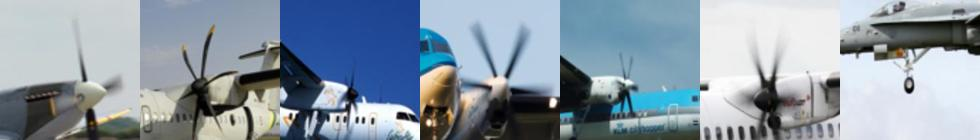} &  \includegraphics[width=0.485\linewidth]{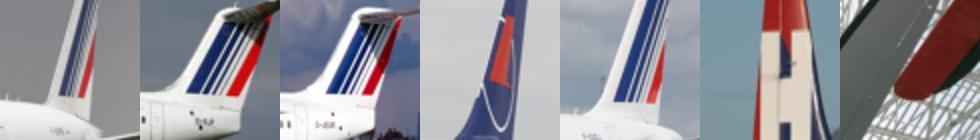}\\
    \includegraphics[width=0.485\linewidth]{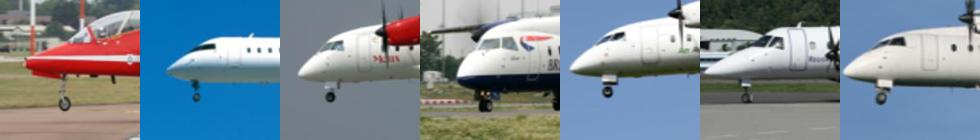} & \includegraphics[width=0.485\linewidth]{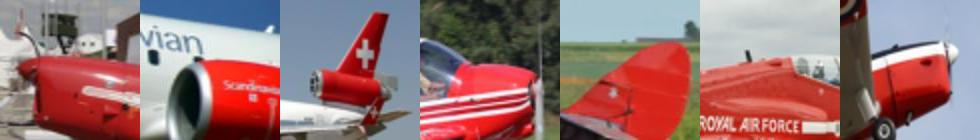}\\
    \includegraphics[width=0.485\linewidth]{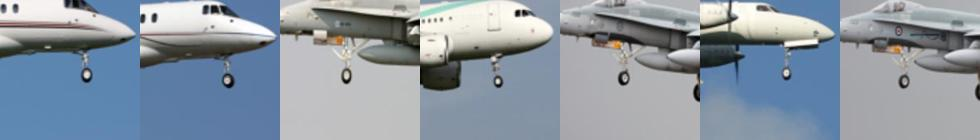} & \includegraphics[width=0.485\linewidth]{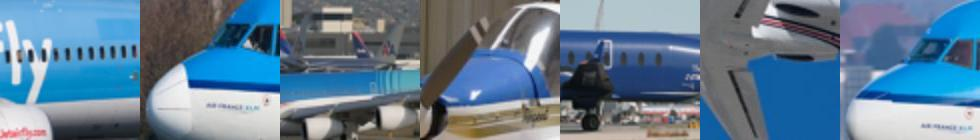}\\
    \includegraphics[width=0.485\linewidth]{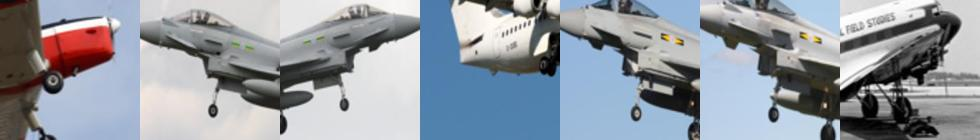} & \includegraphics[width=0.485\linewidth]{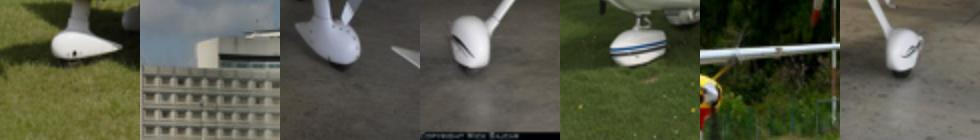}\\
    \includegraphics[width=0.485\linewidth]{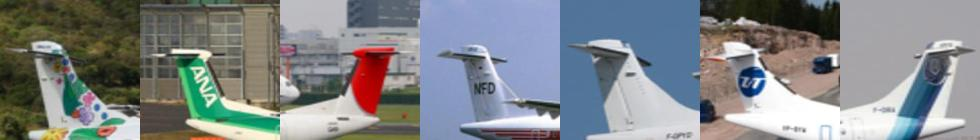} &  \includegraphics[width=0.485\linewidth]{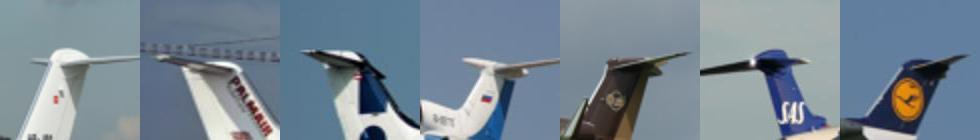}\\
    \includegraphics[width=0.485\linewidth]{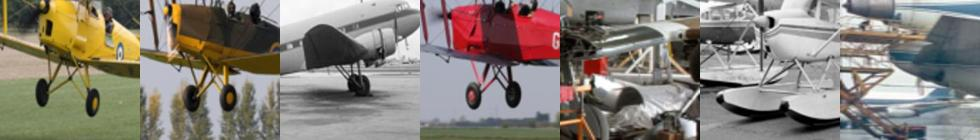} &  \includegraphics[width=0.485\linewidth]{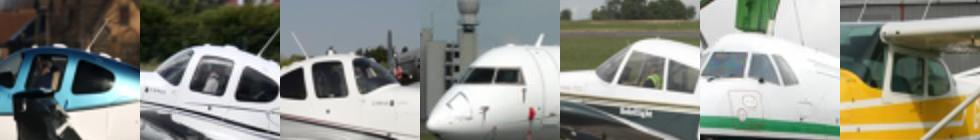}\\
    \end{tabular}
    \caption{\label{fig:bcnn-vis} Patches with the highest activations for several filters of the fine-tuned BCNN(D, M) model on the Aircraft dataset. It can be observed here that each filter is usually activated by a group of patches that have a high-level relationship between themselves - engines, propeller, undercarriage, tail stabilizers, cockpit, a specific colour, etc.}
    \end{center}
    \end{figure}
